# Supplementary material for: Towards an Interpretable Data-driven Trigger System for High-throughput Physics Facilities
Source: arXiv:2104.06622 source file (2021-04-14)
Supplement: Supplementary file 1 [file appendix_sec.tex]

\section*{Appendix}
%%%%%%%%%%%%%%%%%%%%%%%%%%%%%%%%%%%%%

%-----------------------------------------
\paragraph{CMS Open Data}
%-----------------------------------------
For the experiment we use public datasets from the CMS Experiment at the LHC, available in the public CERN Open Data Portal. The Portal represents an exciting opportunity for the general public to access the LHC data for studies such as the trigger optimization presented in this paper.
In particular, we use a simulated dataset of $t\bar{t}$ events \cite{CMSOpenData}, generated for collisions at a centre-of-mass energy of 8 TeV and reconstructed to provide information on the physics objects such as electrons, photons, muons, taus, and jets, as well as their respective masses, transverse momenta, and psuedorapidity. The events also include Boolean values for over 400 different triggers that we have analyzed using the physics information and trigger decisions. The CMS Open Data presents an exciting opportunity for the general public to access the LHC data for studies such as this trigger optimization.
